# Supplementary material for: Robust single-shot 3D fluorescence imaging in scattering media with a simulator-trained neural network
Source: arXiv:2303.12573 source file (2023-12-08)
Supplement: Supplementary file 1 [file SBR_net_Supplementary_OptEx.pdf]

# Supplementary Information: Robust single-shot 3D fluorescence imaging in scattering media with a simulator-trained neural network

Jeffrey Alido[1], Joseph Greene[1], Yujia Xue[1], Guorong Hu[1], Yunzhe Li[1], Mitchell Gilmore[1], Kevin J. Monk[2], Brett T. DiBenedictis[3], Ian G. Davison[2], and Lei Tian[1,3]

[1]Department of Electrical and Computer Engineering, Boston University, Boston, MA 02215, USA.
[2]Department of Biology, Boston University, Boston, MA 02215, USA.
[3]Department of Psychology and Brain Sciences, Boston University, MA 02215, USA.
[4]Department of Biomedical Engineering, Boston University, Boston, MA 02215, USA.
[*]Correspondence: leitian@bu.edu

November 21, 2023

# Contents


**S1 Value noise visualization** **3**

**S2 Statistical comparison of synthetic and experimental data** **4**

**S3 Network architecture** **7**

**S4 Synthetic test data precision and recall** **8**

**S5 Experimental scattering phantoms** **9**
S5.1 Scattering phantom fabrication . . . . . . . . . . . . . . . . . . . . . . . . . . . . . . . . . . . 9

**S6 Experimental scattering phantom reconstruction** **11**

**S7 *Ex-vivo* rodent brain slice experiment** **12**
S7.1 *Ex-vivo* 75 µm thick brain slice reconstruction results . . . . . . . . . . . . . . . . . . . . . . . . 12
S7.2 *Ex-vivo* 75 µm thick brain slice preparation . . . . . . . . . . . . . . . . . . . . . . . . . . . . . 12

**S8 Effect of deep learning factors on SBR-Net generalization to experimental data** **16**

**S9 Variance stabilization speeds up training convergence** **18**

**S10Model-based reconstruction** **20**

**S11Image processing-based background removal** **24**

**S12Light field refocusing** **25**

**S13Detection metrics** **26**

**S14Confocal microscopy** **27**

## S1 Value noise visualization

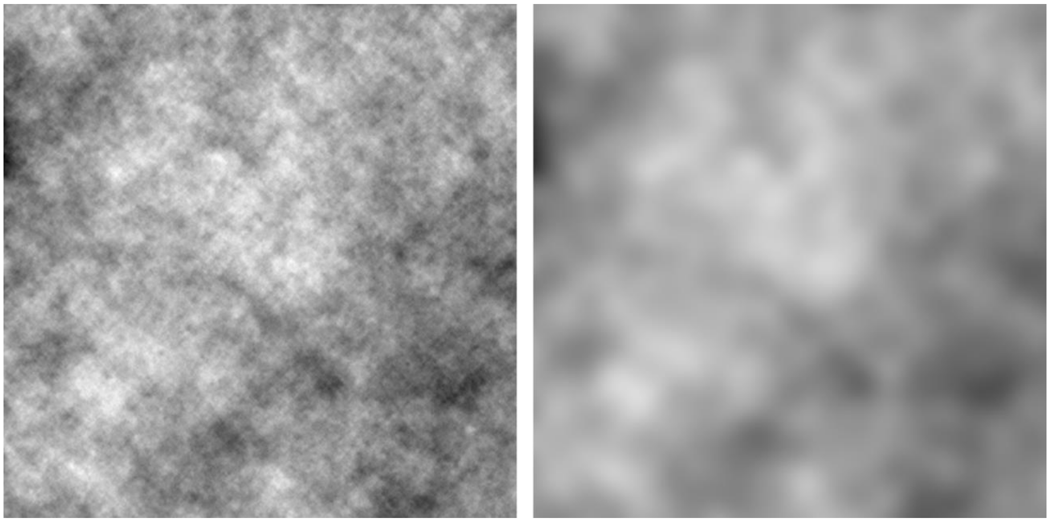

Figure S1: Raw 600 x 600 value noise and its low-pass filtered result using a Gaussian kernel with std of 13 pixels. Note the spatially varying intensities which contributes to different local SBRs.

## S2 Statistical comparison of synthetic and experimental data

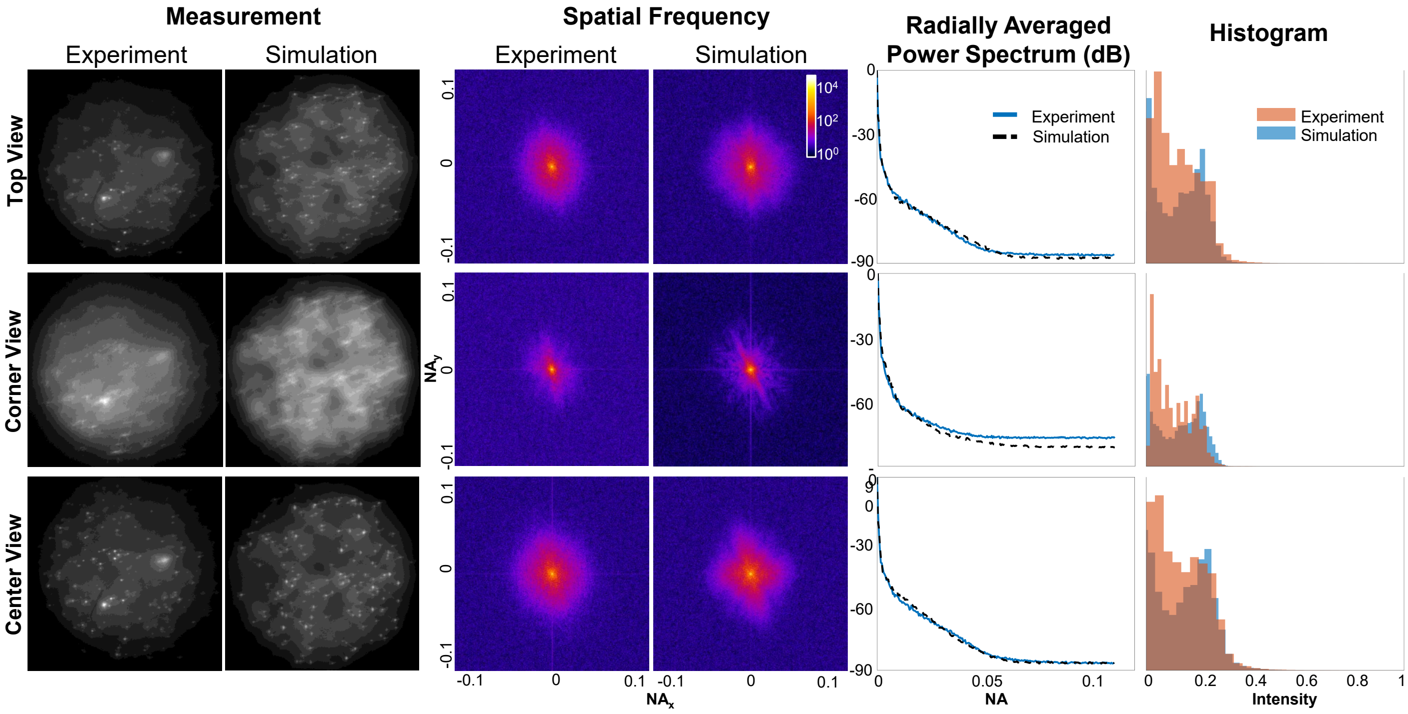


Figure S2: Qualitative and quantitative comparison of synthetic and experimental data for $l_s = 279\,\mu m$. We show the spatial frequency, power spectra, and intensity histograms for different views of a CM$^2$ measurement and observe strong similarities.

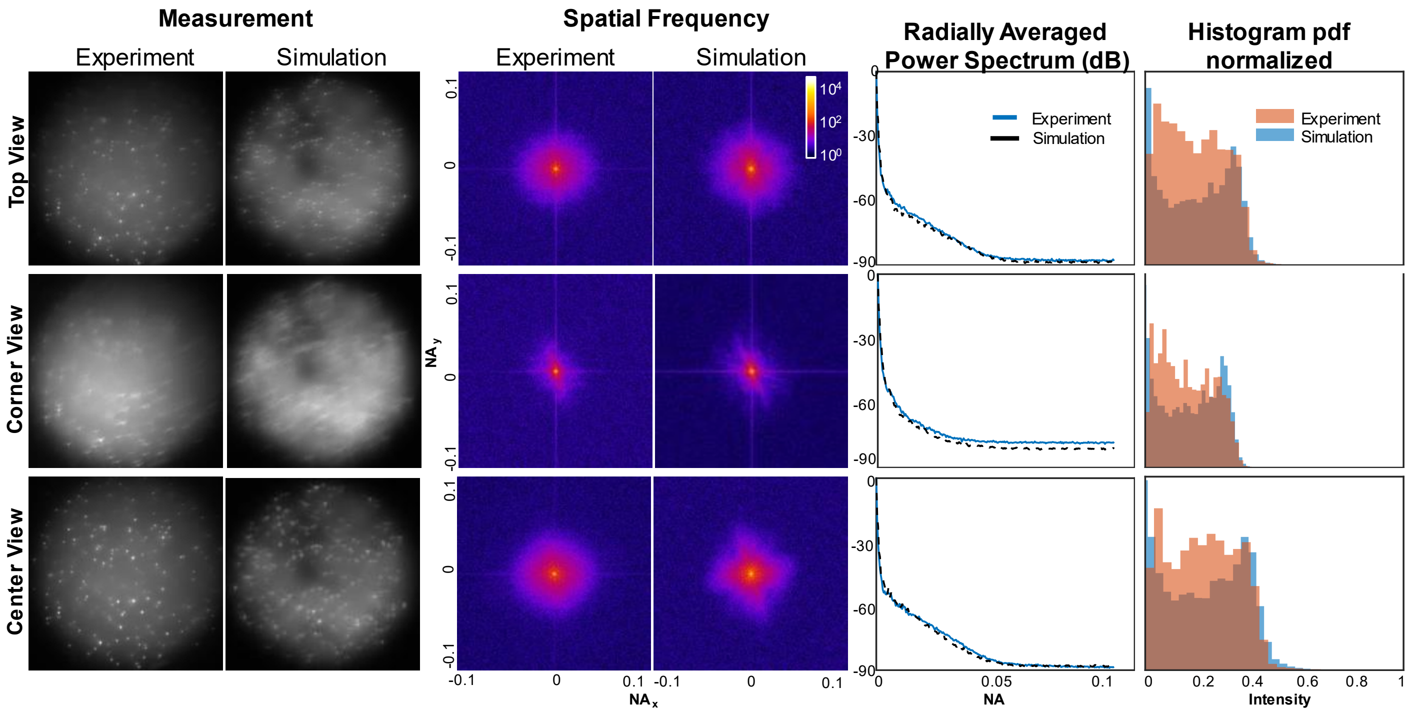


Figure S3: Qualitative and quantitative comparison of synthetic and experimental data for $l_s = 182\,\mu\text{m}$. We show the spatial frequency, power spectra, and intensity histograms for different views of a $\text{CM}^2$ measurement and observe strong similarities.

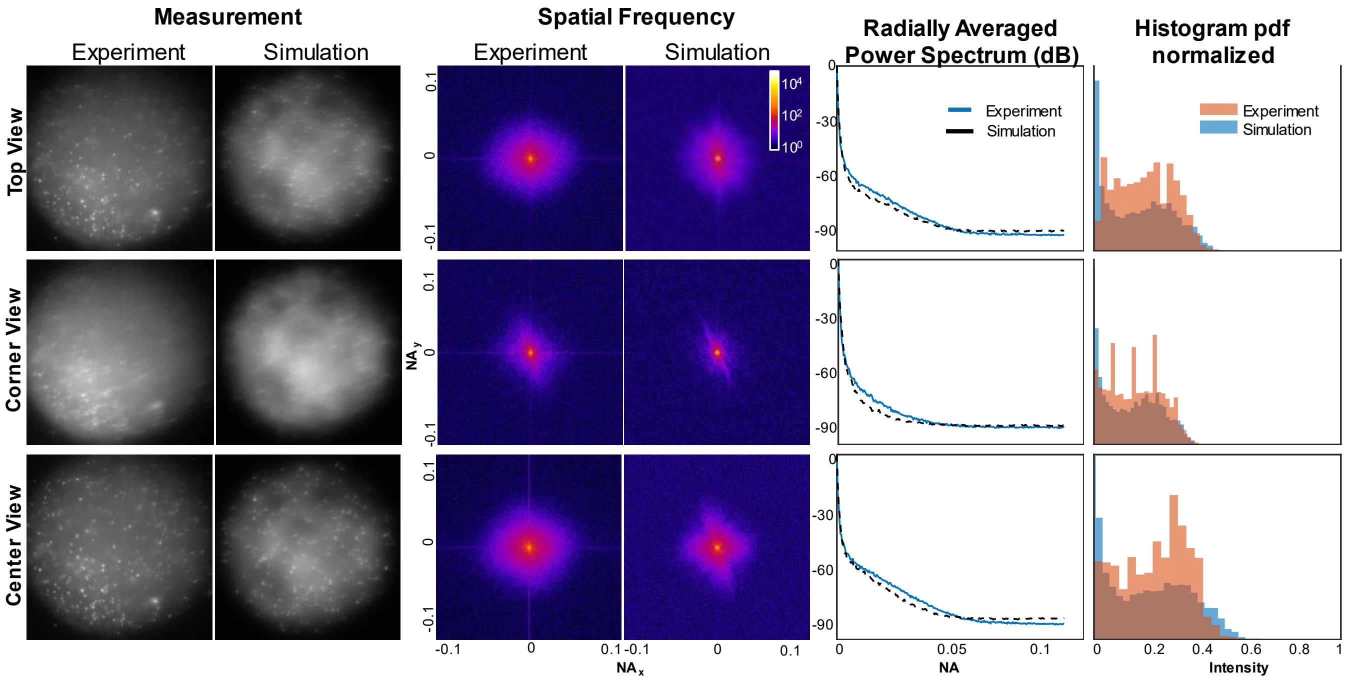


Figure S4: Qualitative and quantitative comparison of synthetic and experimental data for $l_s = 72\,\mu\mathrm{m}$. We show the spatial frequency, power spectra, and intensity histograms for different views of a $\mathrm{CM}^2$ measurement and observe strong similarities.

# S3 Network architecture

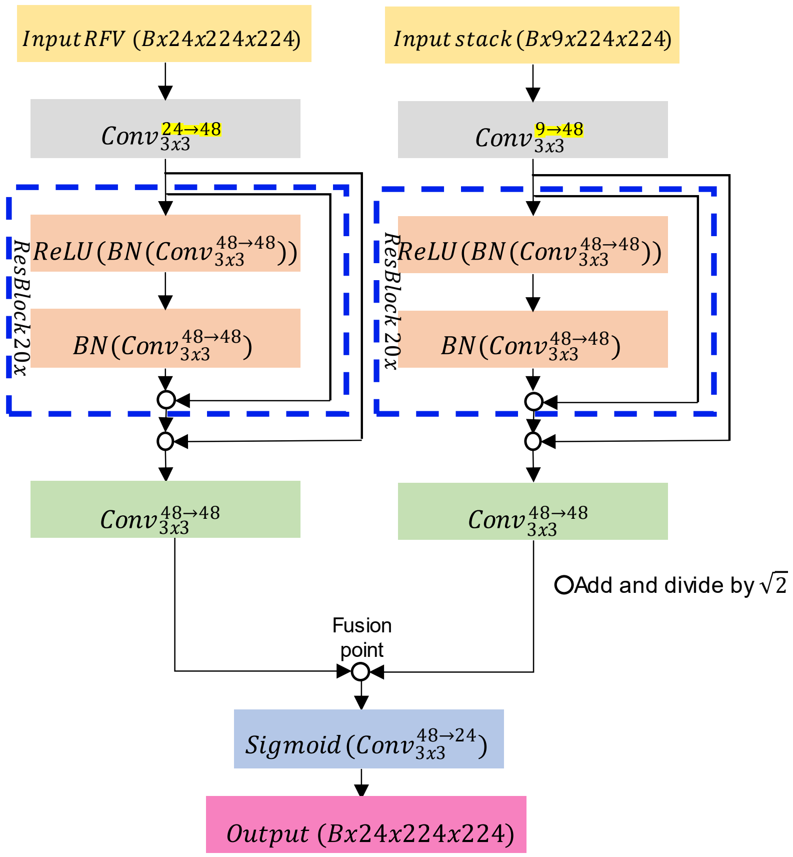


Figure S5: Schematic of our CNN architecture. The superscript of the convolutional layers denotes the number of input channels to the number of output channels, and the subscript denotes the kernel size. BN denotes a batch normalization layer, and B denotes batch size number.

# S4 Synthetic test data precision and recall

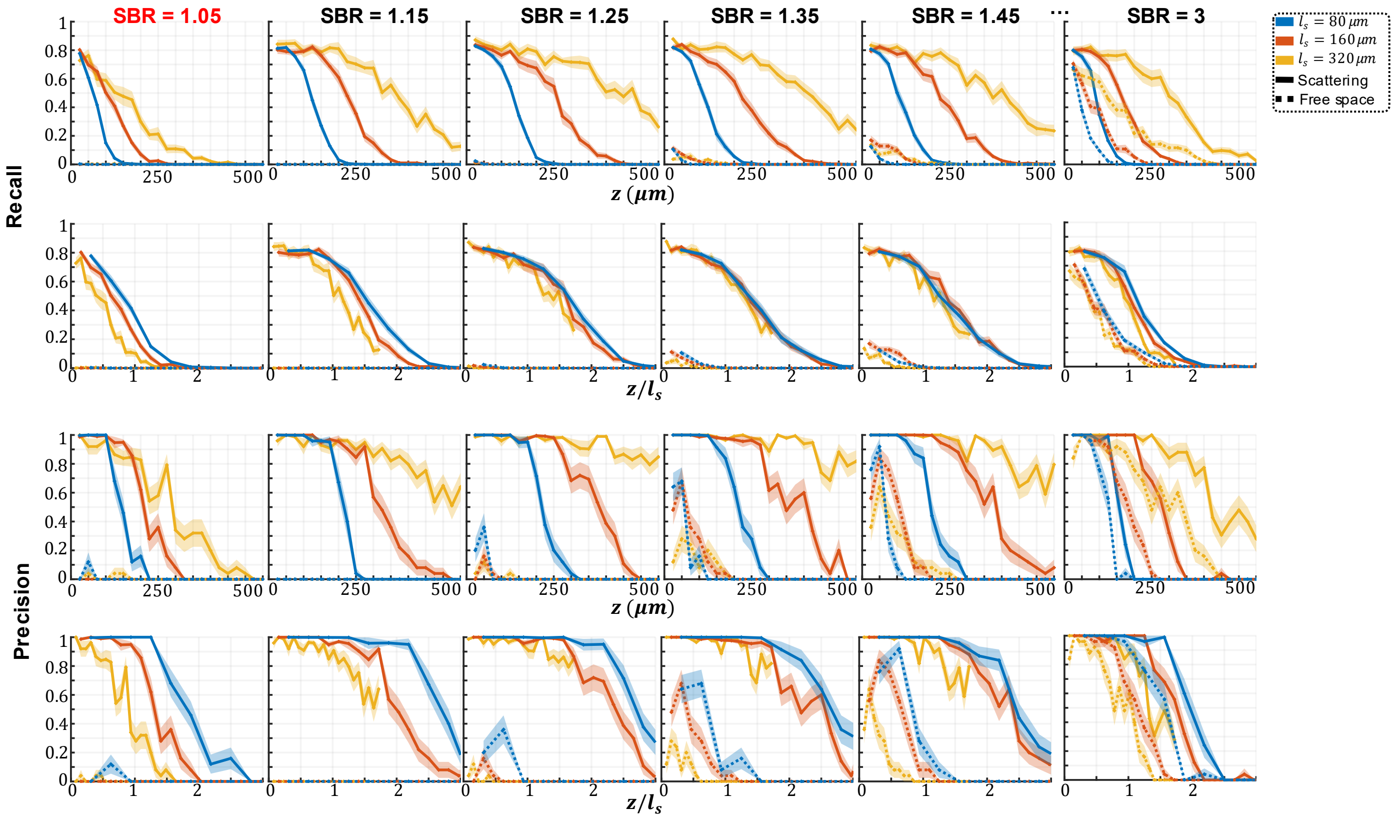


Figure S6: Simulation test data recall and precision metrics. The labeled SBR values are the average SBR values for the particles in the first depth layer before any optical attenuation. Similar to the optical signal, the SBR of a particle would decay exponentially over increasing depth of the particle, which is why we observe a systematic decay of performance for all scattering lengths, as seen in the normalized depths curves. Shaded regions represent standard error over 25 statistical samples. Note that the precision curve for free space peaks at a consistent depth, indicating the network's preference over objects with that depth's system response.

# S5 Experimental scattering phantoms

## S5.1 Scattering phantom fabrication

We fabricate scattering phantoms with bulk scattering and background fluorescence. We control the bulk scattering using a combination of nonfluorescent and green fluorescent $1.1\mu$m polystyrene miscrospheres (i.e. scatterers) (Thermo Fisher Scientific, 5000 Series Polymer Particle Suspension; refractive index, 1.5979), and the background fluorescence with only the green fluorescent $1.1\mu$m microspheres. Our imaging target is a mixture of 10 and $15\mu$m green fluorescent polystyrene beads (Thermo Fisher Scientific, Fluoro-Max Dry Fluorescent Particles, 10 and $15\mu$m), and we neglect their contribution to bulk scattering.

We begin by centrifuging the nonfluorescent scatterer suspension (concentration 10% v/v) in a 1.5 mL microcentrifuge tube at 7000 rpm to separate the polystyrene microspheres from the water, and then pipette out the supernatant leaving only the solid scatterers. We then add 20 $\mu L$ of the fluorescent scatterer suspension (concentration 1% solid), and the imaging targets. Finally, we add 1 mL of uncured polydimethylsiloxane (PDMS) with a 10:1 ratio of base to curing agent (Sylgard 184, Dow Corning Corp., Midland, MI, refractive index, 1.43). We use an ultrasonic probe sonicator (Fisherbrand™ Model 50 Sonic Dismembrator) to thoroughly mix the solution. This mixing process causes a significant amount of cavitation which makes the solution more scattering than desired, so we leave the solution in a vacuum degassing chamber for 20 minutes at a pressure of -30 bar to remove microscopic bubbles and any remaining water. We finally place 2 $\mu L$ of the uncured solution inside a custom 3D printed ring of diameter 2 mm and height 0.5 mm and leave it in an oven at 40C for 4 hours to cure.

To calculate the amount of scatterers needed for a certain bulk scattering length, $\ell_s$, we use Mie theory [1]:

$$\phi = \frac{2d}{3\ell_s Q} \tag{1}$$

where $\phi$ is the concentration (v/v) of scatterers in the medium, $d = 1.1\mu m$ is the diameter of a scatterer, and $Q = 1.9191$ is the scattering efficiency computed with the online Mie scattering calculator [2].

Our target scattering lengths for the phantoms are 75, 200 and $325\mu$m, for which we add 51, 19 and 12 $\mu L$ respectively, of non-fluorescent scatterer suspension to 1 mL of PDMS. After adding 20 $\mu L$ of fluorescent scatterers to each solution, the final scattering length is calculated to be 72, 181, and $279\mu$m, all with an anisotropy factor of $g = 0.95795$. In Fig. S7, we show confocal measurements of all three phantoms to verify that the target scattering length is achieved.

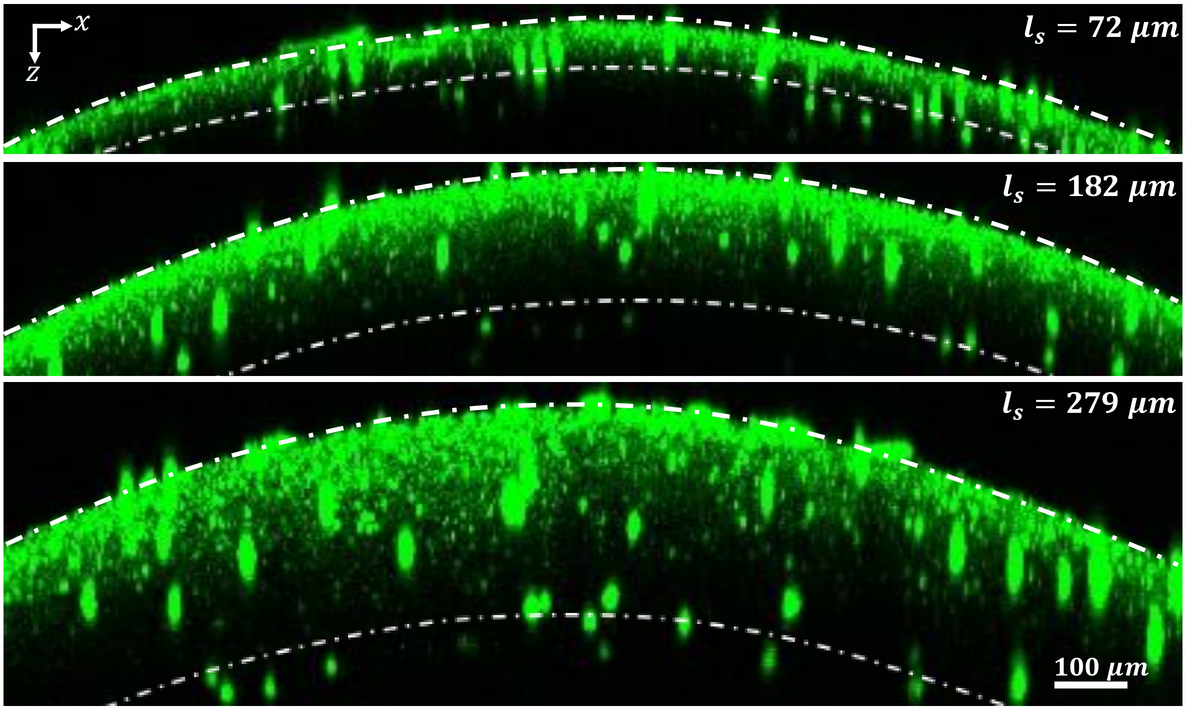


Figure S7: XZ MIP of 1600 µm × 50 µm ROI of the confocal measurements of the scattering phantoms. The dashed-dotted shell represents 1 scattering length from the surface of the phantom. We observe reasonable intensity attenuation that follows Beer-Lambert's law.

# S6 Experimental scattering phantom reconstruction

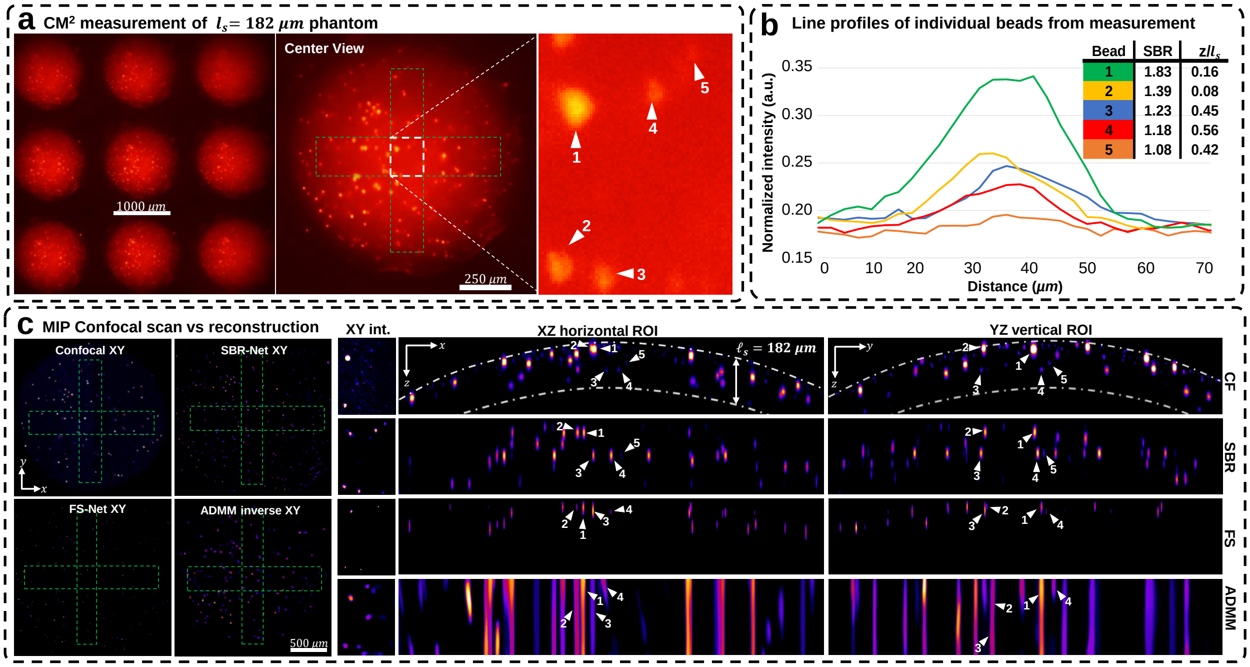


Figure S8: Reconstruction results for $l_s = 182\,\mu\mathrm{m}$ scattering phantom. (a) The raw CM$^2$ measurement with a zoom-in of a small region of interest (ROI) with beads we label to validate reconstruction performance. (b) Line profiles of the labeled beads in the raw CM$^2$ measurement. We list each bead's depth relative to the surface of the phantom as well as their measurement SBRs. (c) MIPs of confocal microscopy 3D measurements, reconstructions with SBR-Net, FS-Net, and the model-based ADMM algorithm. The dashed-dotted line in the confocal XZ/YZ MIPs represent a distance of one scattering length from the surface of the phantom. For this scattering phantom, SBR-Net is able to recover all 5 beads at their correct depth location, which is as deep as over half a scattering length. SBR-Net also reconstructs and localizes a particle with a measurement SBR of 1.08. However, while SBR-Net localizes particles well, it reconstructs them with some inaccuracies in intensity and size. FS-Net and ADMM both fail to reconstruct the particle of the 5 with the lowest SBR of 1.08 and localizes the remaining 4 with poor accuracy. Additionally, the XY MIPs show that SBR-Net provides background rejection for the 2D reconstruction case while retaining low SBR particles, which FS-Net and ADMM remove.

# S7 *Ex-vivo* rodent brain slice experiment

## S7.1 *Ex-vivo* 75 µm thick brain slice reconstruction results

To demonstrate SBR-Net's generalization capability on complex biological samples, we applied the simulator-trained SBR-Net directly on a 75 µm thick fixed section of mouse brain containing fluorescently labelled neurons expressing green fluorescent protein (GFP) delivered with virally mediated approaches. Thickness of the sample is approximately one scattering length of rodent brain tissue [3]. To avoid view-multiplexing in the measurement, we constrain the object FOV to be approximately a circle of 2 mm in diameter by placing a circular field stop directly in front of the sample [4]. The measurement area contains regions with both dense and sparse labelling of neurons. We validated the reconstruction and 3D localization performance of SBR-Net using a confocal microscopy measurement as reference. Comparisons between SBR-Net trained on different SBR ranges, FS-Net and model-based reconstructions are also provided in Figs. S10 and S11.

Our results are shown in Fig. S9, where we demonstrate SBR-Net's optical sectioning and 3D reconstruction performance with two representative ROIs. ROI 1 is of a denser neuron population with neuropil contamination causing low-SBR measurements. ROI 2 is of a sparse region with dimmer fluorescence that also causes low-SBR measurements. SBR-Net is able to reconstruct neurons from their low-SBR measurements as low as 1.05. In addition, SBR-Net can recover the relative depth position of individual neurons, verified by the confocal microscopy measurement.

Furthermore, SBR-Net rejects some background fluorescent structures like dendrites, recovering only the cell bodies. This can be explained by the network being trained on only spherical objects, providing a deep prior that allows the network to reject any other anatomical features. Looking at the overlay between SBR-Net reconstruction and the confocal microscopy measurement, we observe that SBR-Net fails to reconstruct some neurons at the edge of the field of view. This is likely due to the shift-variant aberrations in CM2 system [5] that are exacerbated by scattering leading to distorted features in the measurement that the network has not seen during training, thus it rejects the signals leading to false negatives. We also see that a uniform fluorescent region results in false positive hallucinations. This region is equivalent to a signal with SBR $\approx 1$, where the neurons are indistinguishable from the fluorescence background. These hallucinations can be explained by the fact that this SBR $\approx 1$ structure is unseen by the network resulting in high variance reconstruction behavior.

These results show a promising step towards practical applications of SBR-Net for neural imaging. Recovering signals from their low-SBR measurements may allow improved imaging depth penetration capabilities for lightfield and miniscope experiments, where neuronal signals embedded deeper in scattering tissue tend to have lower SBRs.

## S7.2 *Ex-vivo* 75 µm thick brain slice preparation

Histological sections with GFP-expressing neurons in the bed nucleus of the stria terminalis (BNST) were prepared using viral-mediated techniques. Male C57Bl/6 mice were anesthetized under continuous 2% isoflurane vapor and given preoperative analgesia (buprenorphine and ketoprofen, 0.5 and 5 mg/kg respectively). The head was secured in a digital stereotaxic apparatus (David Kopf Instruments, Tujunga, CA, USA), the skull was exposed with a midline incision and a small craniotomy was performed bilaterally over each injection site. Viral solutions (100-200 nL, pAAV-CAG-GFP, Addgene # 37825-AAVrg) were delivered to the BNST using a pulled glass micropipette (20 µm tip diameter) and a Nanoject II (Drummond) positioned at coordinates 1.0 mm lateral from the midline, 0.4 mm anterior to bregma, and a depth of 4.3 mm from dura. The retrograde virus labeled both local neurons at the injection site in BNST as well as upstream brain areas. Animals recovered for two to three weeks after surgery to allow for viral expression and were then deeply anesthetized with ketamine-xylazine (100 and 15 mg/kg, respectively) and perfused transcardially with 4% paraformaldehyde in phosphate-buffered saline and their brains were subsequently removed, fixed, cryoprotected and sectioned coronally at 75 $\mu$m thickness using a cryostat. Sections were mounted on Superfrost Plus slides (Fisher) and Vectashield mounting medium (Vector Labs). This study was performed in strict accordance with the recommendations in the Guide for the Care and Use of Laboratory Animals of the National Institutes of Health. All animals were handled according to approved Institutional Animal Care and Use Committee (IACUC) protocols (#201800540) of Boston University.

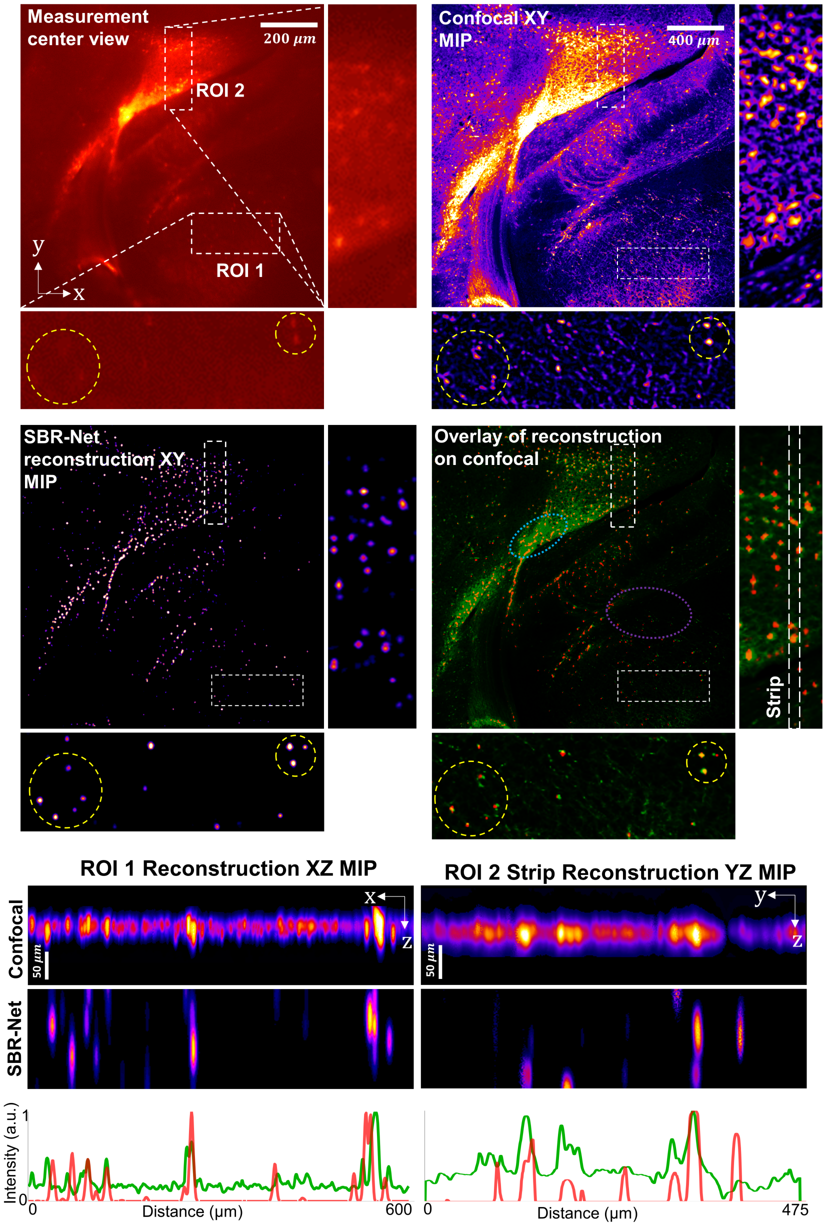


Figure S9: Reconstruction results from an *ex-vivo* rodent brain slice experiment. ROI 1 is of a region of sparse neuron population, and ROI 2 is of a more densely populated region of neurons. We highlight the reconstruction performance of SBR-Net by marking two clusters of low SBR neurons with a yellow circle in ROI 1 for the measurement and reconstruction MIP. The optical contrast of the encircled neurons is low, with SBR less than 1.2. The confocal XY MIPs of the ROIs are processed with rolling ball background subtraction for better visualization of the neurons. The overlay shows the SBR-Net reconstruction in red, and the confocal measurement in green. The light blue dotted oval shows likely false positive reconstructed neurons from a dense nearly uniform region. The purple dotted oval highlights that SBR-Net recovers only spherical neuronal signals and rejects other structures like dendrites. The line profile is the projection of intensity values along each column, which highlights cell body structures from high background in the confocal measurement MIP.

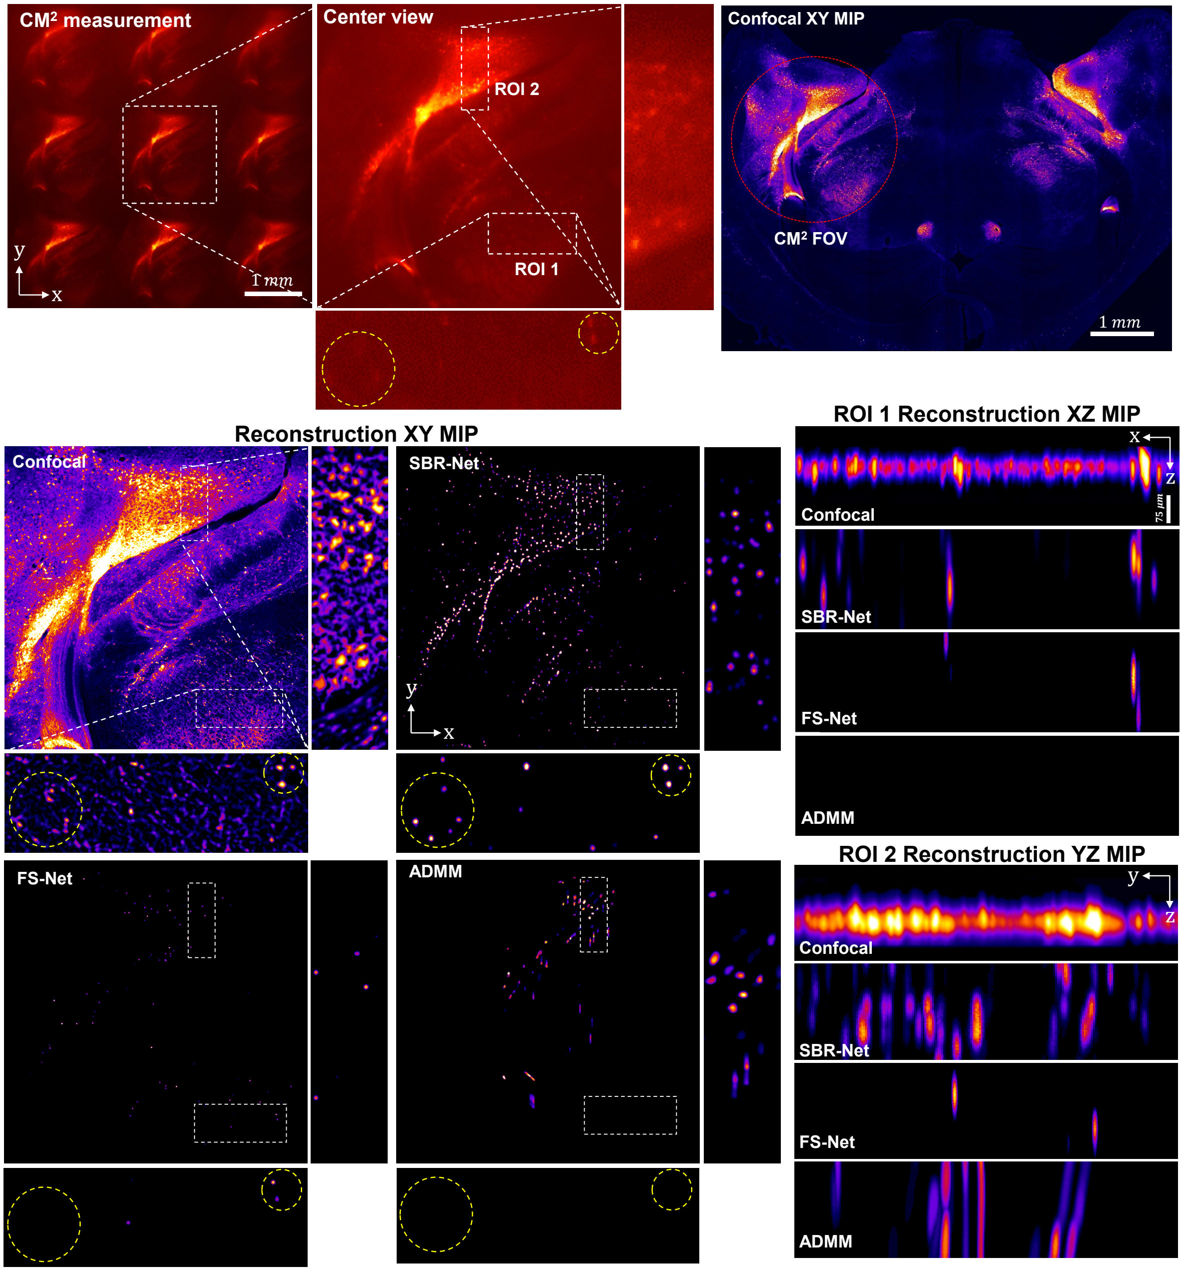


Figure S10: Fixed 75 µm thick brain slice reconstruction results with comparisons with FS-Net and model-based inversion. The raw measurement is shown and low SBR cell body clusters from ROI 1 are encircled with a yellow circle. The reconstruction results for SBR-Net, FS-Net, and model-based reconstruction with ADMM is shown with the confocal microscopy measurements as a benchmark. The XZ and YZ MIPs of the ROIs are given to examine the 3D localization accuracy. The XY MIPs reveal that SBR-Net can recover the low SBR signals in ROI 1, while FS-Net and ADMM cannot. SBR-Net has strong localization performance for both the 2D and 3D localization compared to the other methods. FS-Net fails to reconstruct several emitters, but has no false positives, similar to ADMM. Assessing the YZ MIP of ROI 2, SBR-Net trades off 3D localization accuracy for robustness, as it may have incorrect 3D localization, but strong 2D localization, representing accuracy and robustness, respectively.

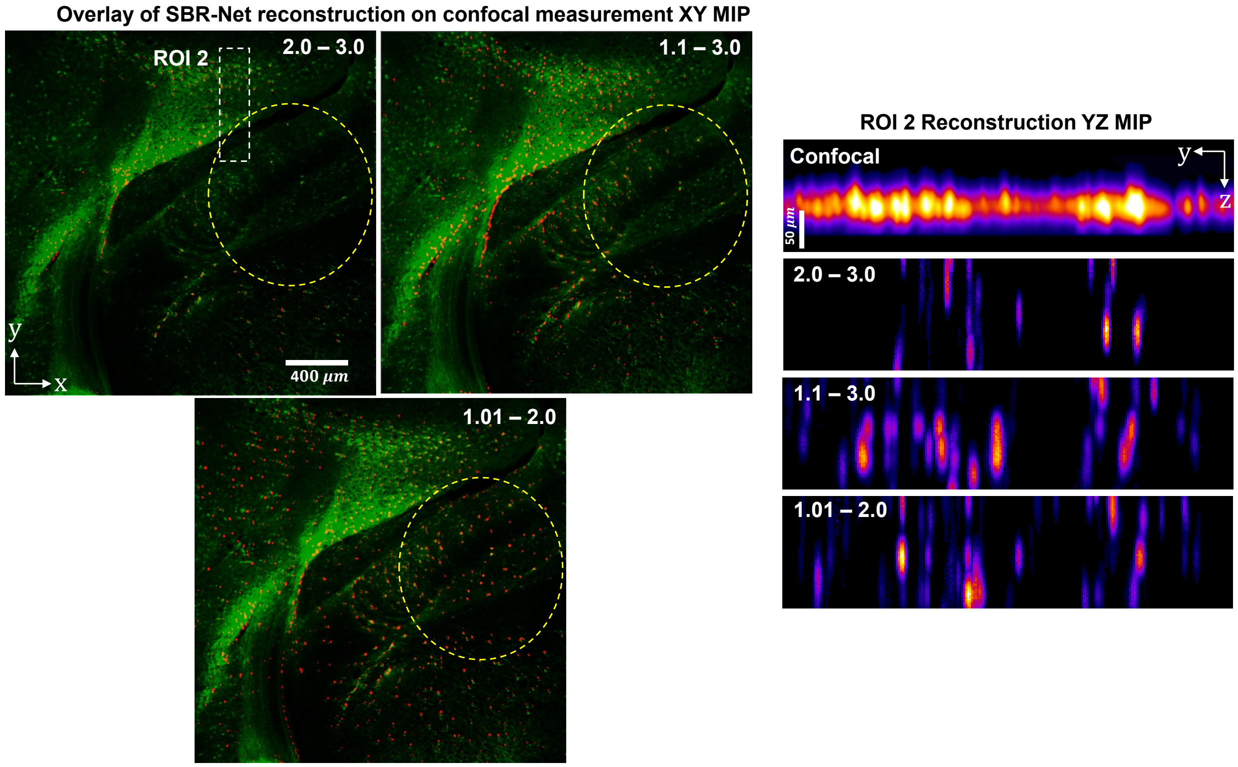


Figure S11: Fixed 75 µm thick brain slice reconstruction results for all three SBR-Nets with different SBR range in training. We observe the robustness-accuracy tradeoff in the sparse labelling region of ROI 1 where SBR-Net (1.1 - 3.0) reconstructs fewer emitters compared to SBR-Net (1.01 - 2.0) (red dashed oval), but has more 3D localization accuracy, as highlighted in the yellow dashed oval. While SBR-Net (1.01 – 2.0) may recover more in the 2D reconstruction of the XY MIP, the 3D localization performance is poor, demonstrating a tradeoff of accuracy for robustness. For the denser labelling region of ROI 2, SBR-Net (2.0 - 3.0) performs poorly in robustness, recovering fewer emitters, but has better localization accuracy (light blue dashed oval). As a separate note, SBR-Net (1.01 - 2.0) outperforms the other two networks in XY localization as seen in the XY MIP overlays on confocal measurements.

## S8 Effect of deep learning factors on SBR-Net generalization to experimental data

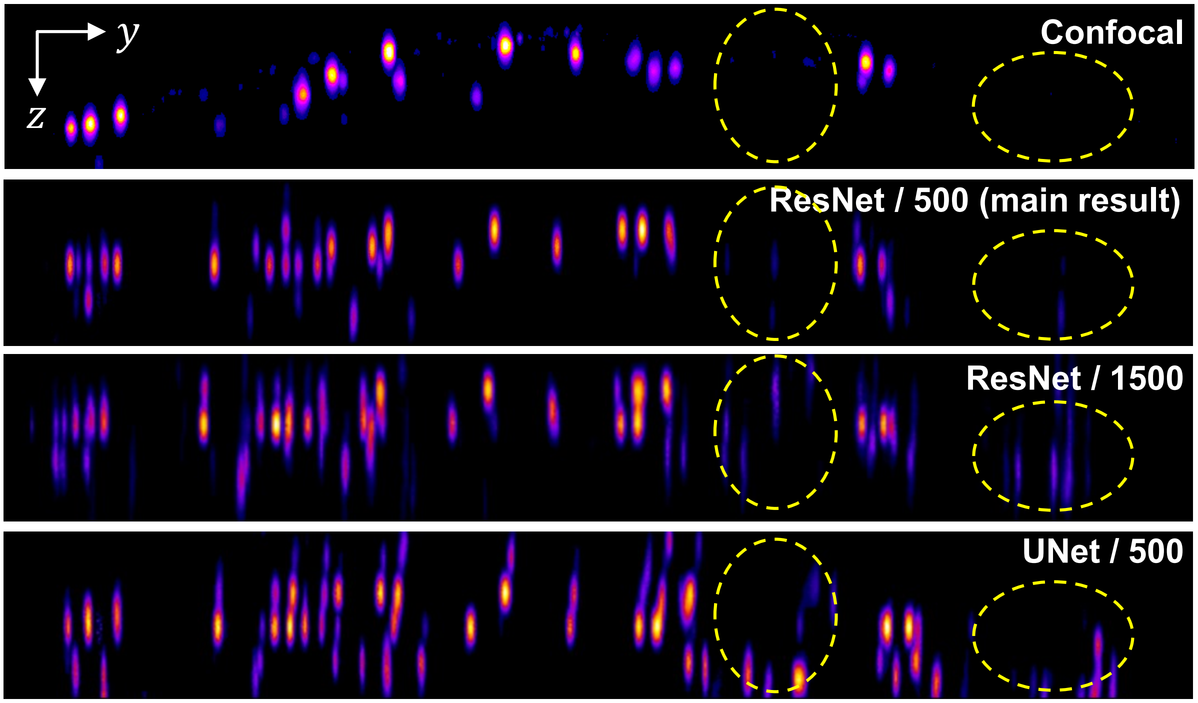


Figure S12: YZ MIPs of the SBR-Net reconstruction results on the 72 µm phantom SBR-Net trained on 1500 unique training data pairs generalizes more poorly to experimental data compared to the one trained with 500 unique pairs, as seen by more hallucination artifacts. We also see a similar behavior for the UNet-based SBR-Net with more network parameters.

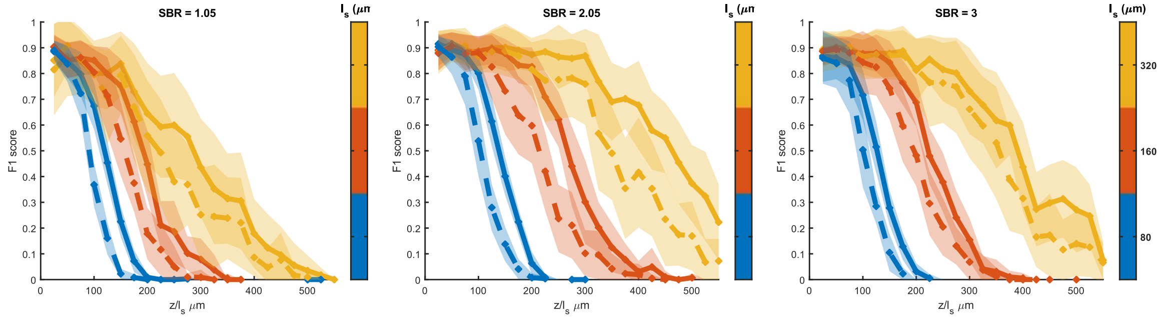


Figure S13: F1 scores for UNet-based (solid) and ResNet-based (dashed) architectures for data with different peak SBRs (1.05, 2.05, 3.0) across 3 scattering lengths (320, 160, 80 µm).

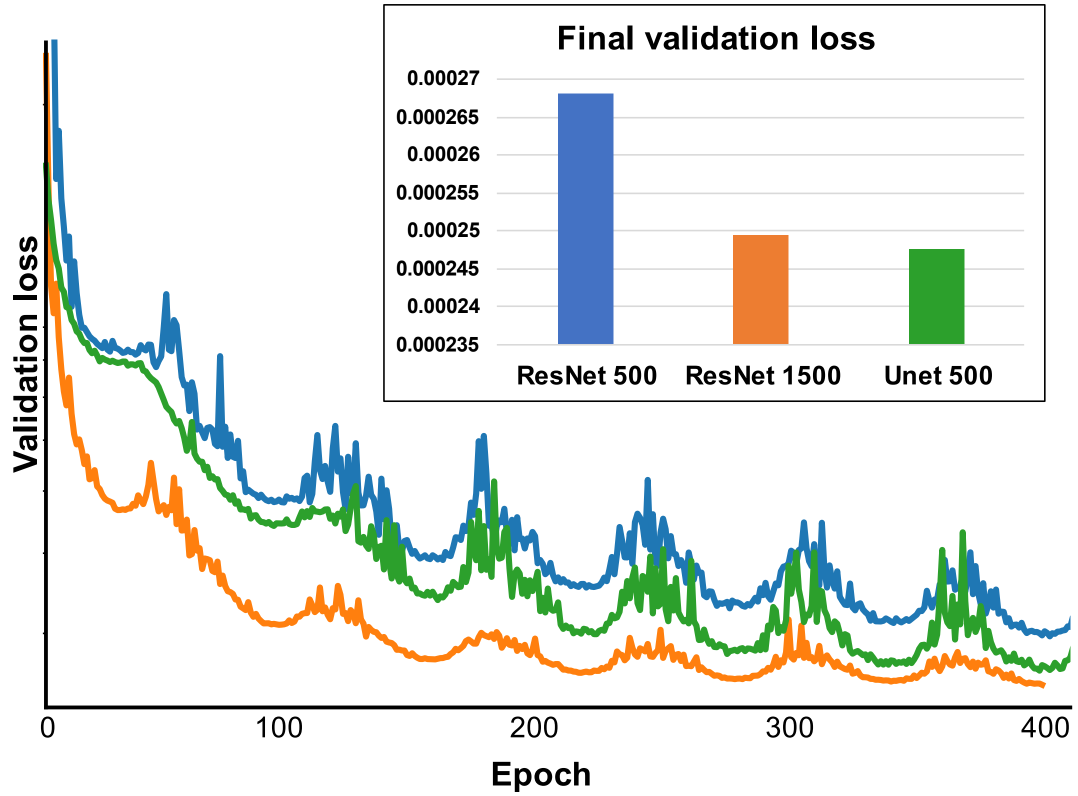


Figure S14: Validation loss for SBR-Net (500 pairs), SBR-Net (1500 pairs), and UNet-based SBR-Net.

# S9 Variance stabilization speeds up training convergence

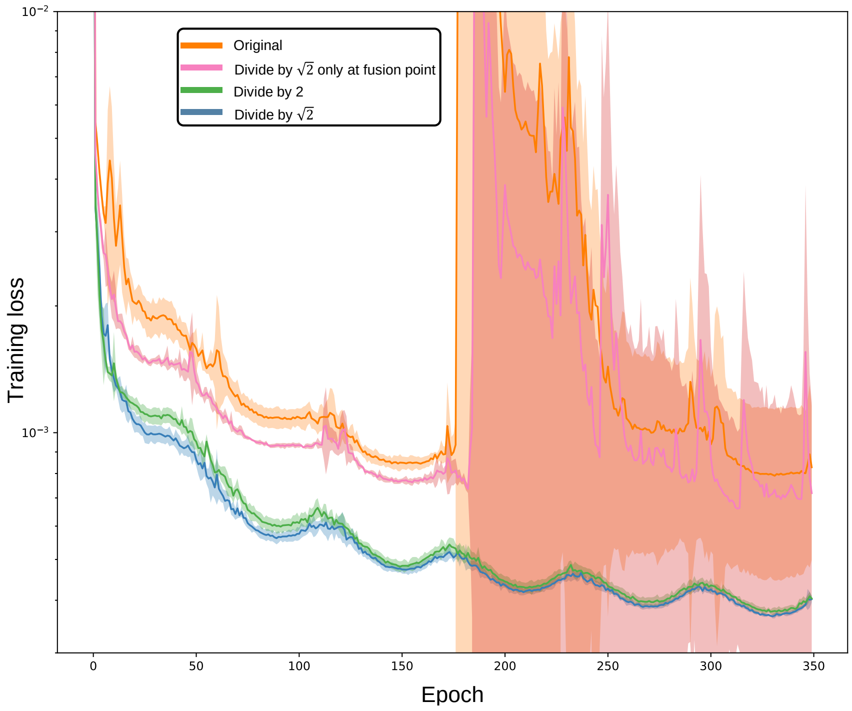


Figure S15: Variance stabilization speeds up training convergence by a factor of 7. Shading represents standard deviation for 5 training experiments.

When two independent random variables, $X$ and $Y$ are added, the variance of the sum, $Z$ is

$$\begin{aligned} Var[Z] &= Var[aX] + Var[bY] \\ &= a^2 Var[X] + b^2 Var[Y]. \end{aligned} \tag{2}$$

In our ResNet-based CNN architecture, there are many channels with random elements being added, and we can safely assume they are independent during the first few epochs. When this happens, the variance grows rapidly over the 20 ResBlocks as well as with the branch fusion. The consequence is that the forward propagation signal has a significantly large range of values which may saturate and flood the sigmoid function at the end of the network, resulting in less meaningful backpropagation signals that lead to slower convergence to local minima.

In our case, $a$ and $b$ are equal to 1, and $X$ and $Y$ have the same variance, $\sigma^2$, so the variance of the forward propagation signal doubles after every ResBlock. We initialize the weights according to Kaiming He initialization [6], $W \sim \mathcal{N}(0, \frac{2}{n_l})$, where $W$ is an element of the CNN layer and $n_l$ is the number of elements in that layer. By the end, the output magnifies the input variance by $2^{21}$ (20 residual connections and one branch fusion). To ensure that the variance of the forward propagation signal does not explode and that we can take advantage of He initialization to its fullest in a ResNet-type architecture, we must ensure that the variance of the forward propagation signal is stabilized, meaning that the variance of the sum of two channels in the network architecture is the same as the variance of the channels that are being summed. From Equation 2, we see the solution is to divide the sum by $\sqrt{2}$:

$$Var[Z] = Var\left[\frac{X+Y}{\sqrt{2}}\right] = \frac{Var[X] + Var[Y]}{\sqrt{2}^2} = \frac{\sigma^2 + \sigma^2}{2} = \sigma^2. \tag{3}$$

Thus, for every part of our network where two channels are being added (i.e. the residual connections and the branch fusion), we simply divide the sum by $\sqrt{2}$. In general, channels being fused together with addition should have the sum divided by the square root of the number of channels being fused together.

We experiment with 4 different network structures: without variance stabilization, with variance stabilization for every residual connection and the branch fusion, variance stabilization at only the branch fusion point with the original ResNet residual connections, and dividing by 2 for all residual connections and the branch fusion. Figure S15 show the convergence of the training loss over epochs, and we see that the architecture with variance stabilization is optimal. It takes the architecture with variance stabilization 7 times faster to reach the same training loss as it does for the original architecture without variance stabilization. The original architecture and the one where only the branch fusion point has been divided by $\sqrt{2}$ are prone to severely non-optimal model weights due to the large variance of the forward propagation signal combined with warm restarts of the learning rate.

# S10 Model-based reconstruction

This section adopts the following notation: bolded uppercase letters denote operators, a superscript of $H$ denotes the Hermitian adjoint of the operator, bolded lowercase letters denote vectors, $\top$ denotes the transpose, and unbolded characters denote scalars.

We use the free space model for the CM$^2$ imaging system and invert the scattering measurements that have undergone background removal, both of which have been reported in our previous study [4]. Briefly, the imaging system is a slice-wise shift-invariant model, followed by a cropping operator, $\mathbf{C}$, to account for the finite area of the camera sensor:

$$\mathbf{y} = \mathbf{CAx} \tag{4}$$

where $\mathbf{x} = [\mathbf{x}_1, \mathbf{x}_2, \ldots, \mathbf{x}_n]$ is the discretized 3D object with $n$ number of axial slices and $\mathbf{A} = [\mathbf{A}_1, \mathbf{A}_2, \ldots, \mathbf{A}_n]$ is the slice-wise discrete forward model such that $\mathbf{Ax} = \sum_{i=1}^{n} \mathbf{A}_i \mathbf{x}_i$, projecting all the depth-wise 2D measurements onto the camera sensor plane.

The inverse problem is highly ill-posed due to the 2D to 3D dimension mismatch, so we incorporate sparsity priors in the spatial and gradient domain of the object and solve the following optimization problem:

$$\hat{\mathbf{x}} = \underset{\mathbf{x} \geq 0}{\arg\min} \frac{1}{2} \|\mathbf{y} - \mathbf{CAx}\|_2^2 + \tau_1 \|\mathbf{x}\|_1 + \tau_2 \|\mathbf{Dx}\|_1 \tag{5}$$

where $\mathbf{D}$ is the 3D finite difference operator, and $\tau_1$ and $\tau_2$ are manually tuned non-negative regularization parameters. We use a spatial sparsity prior because our objects are beads or neurons in a volume, where there will be many more zero-valued voxels than nonzero-valued voxels. The 3D total variation prior is widely used for natural objects.

We solve this optimization problem using the alternating direction method of multipliers (ADMM) [4,7,8]. The first step is to perform variable splitting by setting $\mathbf{u} = \mathbf{Ax}$, $\mathbf{v} = \mathbf{x}$, $\mathbf{w} = \mathbf{Dx}$, $\mathbf{z} = \mathbf{x}$, and adding their corresponding constraint sets to the objective. We rewrite the optimization problem as

$$\begin{aligned} \underset{\mathbf{x}, \mathbf{u}, \mathbf{v}, \mathbf{w}, \mathbf{z}}{\arg\min} \quad & \frac{1}{2} \|\mathbf{y} - \mathbf{Cu}\|_2^2 + \tau_1 \|\mathbf{v}\|_1 + \tau_2 \|\mathbf{w}\|_1 \\ \text{s.t.} \quad & \mathbf{u} = \mathbf{Ax}, \\ & \mathbf{v} = \mathbf{x}, \\ & \mathbf{w} = \mathbf{Dx}, \\ & \mathbf{z} = \mathbf{x}, \\ & \mathbf{z} \geq 0. \end{aligned} \tag{6}$$

The next step is to form the augmented Lagrangian to make the optimization unconstrained:

$$\begin{aligned} \mathcal{L}(\{\mathbf{u}, \mathbf{v}, \mathbf{w}, \mathbf{z}, \mathbf{x}\}, \{\boldsymbol{\kappa}, \boldsymbol{\lambda}, \boldsymbol{\mu}, \boldsymbol{\nu}\}) = & \frac{1}{2} \|\mathbf{y} - \mathbf{Cu}\|_2^2 + \tau_1 \|\mathbf{v}\|_1 + \tau_2 \|\mathbf{w}\|_1 \\ & + \frac{\rho_1}{2} \|\mathbf{Ax} - \mathbf{u}\|_2^2 + \boldsymbol{\kappa}^\top (\mathbf{Ax} - \mathbf{u}) \\ & + \frac{\rho_2}{2} \|\mathbf{x} - \mathbf{v}\|_2^2 + \boldsymbol{\lambda}^\top (\mathbf{x} - \mathbf{v}) \\ & + \frac{\rho_3}{2} \|\mathbf{Dx} - \mathbf{w}\|_2^2 + \boldsymbol{\mu}^\top (\mathbf{Dx} - \mathbf{w}) \\ & + \frac{\rho_4}{2} \|\mathbf{x} - \mathbf{z}\|_2^2 + \boldsymbol{\nu}^\top (\mathbf{x} - \mathbf{z}) \\ & + \mathcal{I}_+(\mathbf{z}) \end{aligned} \tag{7}$$

where $\rho_i$ are positive penalty parameters, $(\boldsymbol{\kappa}, \boldsymbol{\lambda}, \boldsymbol{\mu}, \boldsymbol{\nu})$ are the Lagrangian multipliers, or dual variables, and $\mathcal{I}_+(\mathbf{z})$ is the non-negativity barrier function defined as

$$\mathcal{I}_+(z) = \begin{cases} \infty & z < 0 \\ 0 & z \geq 0. \end{cases} \tag{8}$$

The dual function is defined as

$$g(\boldsymbol{\kappa}, \boldsymbol{\lambda}, \boldsymbol{\mu}, \boldsymbol{\nu}) = \inf_{\mathbf{u},\mathbf{v},\mathbf{w},\mathbf{z},\mathbf{x}} \mathcal{L}(\{\mathbf{u}, \mathbf{v}, \mathbf{w}, \mathbf{z}, \mathbf{x}\}, \{\boldsymbol{\kappa}, \boldsymbol{\lambda}, \boldsymbol{\mu}, \boldsymbol{\nu}\}) \tag{9}$$

and solving Eq. 5 is equivalent to solving the *dual problem*:

$$\max_{\boldsymbol{\kappa},\boldsymbol{\lambda},\boldsymbol{\mu},\boldsymbol{\nu}} g(\boldsymbol{\kappa}, \boldsymbol{\lambda}, \boldsymbol{\mu}, \boldsymbol{\nu}). \tag{10}$$

The optimization problem is then a saddle point problem solved by iteratively alternating between a minimization step of the primal variables, followed by a maximization step of the dual variables,

$$\max_{\boldsymbol{\kappa},\boldsymbol{\lambda},\boldsymbol{\mu},\boldsymbol{\nu}} \min_{\mathbf{u},\mathbf{v},\mathbf{w},\mathbf{z},\mathbf{x}} \mathcal{L}(\{\mathbf{u}, \mathbf{v}, \mathbf{w}, \mathbf{z}, \mathbf{x}\}, \{\boldsymbol{\kappa}, \boldsymbol{\lambda}, \boldsymbol{\mu}, \boldsymbol{\nu}\}). \tag{11}$$

We update the dual variables using gradient ascent where the step size is the corresponding penalty parameter. Using calculus, we compute the update steps for the primal variables. The algorithm is as follows:

$$
\begin{aligned}
\mathbf{u}_{k+1} &= \arg\min_{\mathbf{u}} \left\{ \frac{1}{2}\|\mathbf{y} - \mathbf{C}\mathbf{u}\|_2^2 + \frac{\rho_1}{2}\|\mathbf{A}\mathbf{x}_k - \mathbf{u}\|_2^2 + \boldsymbol{\kappa}_k^\top(\mathbf{A}\mathbf{x}_k - \mathbf{u}) \right\} \\
&= (\mathbf{C}^H\mathbf{C} + \rho_1\mathbf{I})^{-1}(\mathbf{C}^H\mathbf{y}_k + \boldsymbol{\kappa}_k + \rho_1\mathbf{A}\mathbf{x}_k) \\
\mathbf{v}_{k+1} &= \arg\min_{\mathbf{v}} \left\{ \tau_1\|\mathbf{v}\|_1 + \frac{\rho_2}{2}\|\mathbf{x}_k - \mathbf{v}\|_2^2 + \boldsymbol{\lambda}_k^\top(\mathbf{x}_k - \mathbf{v}) \right\} \\
&= \arg\min_{\mathbf{v}} \left\{ \frac{\tau_1}{\rho_2}\|\mathbf{v}\|_1 + \frac{1}{2}\|\mathbf{x}_k - \mathbf{v} + \frac{\boldsymbol{\lambda}_k}{\rho_2}\|_2^2 + \cancel{\frac{\boldsymbol{\lambda}_k^\top\boldsymbol{\lambda}_k}{\rho_2^2}} \right\} \\
&= \mathrm{Prox}_{\frac{\tau_1}{\rho_2}\|\cdot\|_1}\left(\mathbf{x}_k - \frac{\boldsymbol{\lambda}_k}{\rho_2}\right) \\
&= \mathcal{S}_{\frac{\tau_1}{\rho_2}}\left(\mathbf{x}_k - \frac{\boldsymbol{\lambda}_k}{\rho_2}\right) \\
\mathbf{w}_{k+1} &= \arg\min_{\mathbf{w}} \left\{ \tau_2\|\mathbf{w}\|_1 + \frac{\rho_3}{2}\|\mathbf{D}\mathbf{x}_k - \mathbf{w}\|_2^2 + \boldsymbol{\mu}_k^\top(\mathbf{D}\mathbf{x}_k - \mathbf{w}) \right\} \\
&= \arg\min_{\mathbf{w}} \left\{ \frac{\tau_2}{\rho_3}\|\mathbf{w}\|_1 + \frac{1}{2}\|\mathbf{D}\mathbf{x}_k - \mathbf{w} + \frac{\boldsymbol{\mu}_k}{\rho_3}\|_2^2 + \cancel{\frac{\boldsymbol{\mu}_k^\top\boldsymbol{\mu}_k}{\rho_3^2}} \right\} \\
&= \mathrm{Prox}_{\frac{\tau_2}{\rho_3}\|\cdot\|_1}\left(\mathbf{D}\mathbf{x}_k - \frac{\boldsymbol{\mu}_k}{\rho_3}\right) \\
&= \mathcal{S}_{\frac{\tau_2}{\rho_3}}\left(\mathbf{D}\mathbf{x}_k - \frac{\boldsymbol{\mu}_k}{\rho_3}\right) \\
\mathbf{z}_{k+1} &= \arg\min_{\mathbf{z}} \left\{ \frac{\rho_4}{2}\|\mathbf{x}_k - \mathbf{z}\|_2^2 + \boldsymbol{\nu}_k^\top(\mathbf{x}_k - \mathbf{z}) + \mathcal{I}_+(\mathbf{z}) \right\} \\
&= \arg\min_{\mathbf{z}} \left\{ \mathcal{I}_+(\mathbf{z}) + \|\mathbf{x}_k - \mathbf{z} + \frac{\boldsymbol{\nu}_k}{\rho_4}\|_2^2 + \cancel{\frac{\boldsymbol{\nu}_k^\top\boldsymbol{\nu}_k}{\rho_4}} \right\} \\
&= \max\left(\mathbf{0}, \mathbf{x}_k + \frac{\boldsymbol{\nu}_k}{\rho_4}\right) \\
\mathbf{x}_{k+1} &= \arg\min_{\mathbf{x}} \left\{ \frac{\rho_1}{2}\|\mathbf{A}\mathbf{x} - \mathbf{u}_{k+1}\|_2^2 + \boldsymbol{\kappa}_{k+1}^\top(\mathbf{A}\mathbf{x} - \mathbf{u}_{k+1}) + \frac{\rho_2}{2}\|\mathbf{x} - \mathbf{v}_{k+1}\|_2^2 + \boldsymbol{\lambda}_{k+1}^\top(\mathbf{x} - \mathbf{v}_{k+1}) \right. \\
&\qquad \left. + \frac{\rho_3}{2}\|\mathbf{D}\mathbf{x} - \mathbf{w}_{k+1}\|_2^2 + \boldsymbol{\mu}_{k+1}^\top(\mathbf{D}\mathbf{x} - \mathbf{w}_{k+1}) + \frac{\rho_4}{2}\|\mathbf{x} - \mathbf{z}_{k+1}\|_2^2 + \boldsymbol{\nu}_{k+1}^\top(\mathbf{x} - \mathbf{z}_{k+1}) \right\} \\
&= \frac{\mathbf{A}^H(\rho_1\mathbf{u}_{k+1} - \boldsymbol{\kappa}_k) + \mathbf{D}^H(\rho_3\mathbf{w}_{k+1} - \boldsymbol{\mu}_k) + \rho_2\mathbf{v}_{k+1} + \rho_4\mathbf{z}_{k+1} + \boldsymbol{\nu}_k - \boldsymbol{\lambda}_k}{\rho_1\mathbf{A}^H\mathbf{A} + \rho_2\mathbf{I} + \rho_3\mathbf{D}^H\mathbf{D} + \rho_4\mathbf{I}} \\
\boldsymbol{\kappa}_{k+1} &= \boldsymbol{\kappa}_k + \rho_1(\mathbf{A}\mathbf{x}_{k+1} - \mathbf{u}_{k+1}) \\
\boldsymbol{\lambda}_{k+1} &= \boldsymbol{\lambda}_k + \rho_2(\mathbf{x}_{k+1} - \mathbf{v}_{k+1}) \\
\boldsymbol{\mu}_{k+1} &= \boldsymbol{\mu}_k + \rho_3(\mathbf{D}\mathbf{x}_{k+1} - \mathbf{w}_{k+1}) \\
\boldsymbol{\nu}_{k+1} &= \boldsymbol{\nu}_k + \rho_4(\mathbf{x}_{k+1} - \mathbf{z}_{k+1})
\end{aligned}
\tag{12}
$$

where $k$ is the iteration step and $\mathrm{Prox}_{\alpha f}$ refers to the proximal operator of function $\alpha f$. In our case, $\alpha f$, is the $l1$ norm with regularization parameter, $\alpha$. This is equal to the soft-thresholding function, $\mathcal{S}_\alpha$.

The adjoint of the cropping operator is zero-padding outside the sensor region, and $\mathbf{C}^H\mathbf{C}$ may be interpreted as a binary mask with a rectangle of ones in the center corresponding to the size of the sensor, so that the matrix is diagonalized and easily invertible. The finite difference operator, $\mathbf{D}$, is implemented using the forward difference operator (i.e. $x_{i+1} - x_i$), and its adjoint is the backwards difference operator, (i.e. $x_{i-1} - x_i$). We assume a circular boundary for simplicity. $\mathbf{D}^H\mathbf{D}$ may be implemented by using a convolutional kernel to carry out the $\mathbf{D}$ and $\mathbf{D}^H$ operator. The forward model operator, $\mathbf{A}$, the 3D finite difference operator $\mathbf{D}$, and their adjoints were carried out in the Fourier domain for computational efficiency and ease of invertibility when the matrix is diagonalized. Our implementation may be found in our open source GitHub [9].

We find the optimal regularization parameters through grid search and visually inspecting the most accurate reconstructions across all three scattering phantoms. The values are $\tau_1 = 0.01$, $\tau_2 = 0.005$, and we keep the penalty parameters $\rho_1 = \rho_2 = \rho_3 = \rho_4 = 1$. The algorithm is carried out in MATLAB R2019b using a Intel Xeon E5-1620 v4 3.5GHz CPU and takes approximately 1.45 hours for one volume.

## S11 Image processing-based background removal

Background removal was carried out in three steps using MATLAB R2019b. The first step is to perform image erosion (`imerode`) on the raw measurement with a disk structural element with radius approximately the same as that of the target structure, which is 5 pixels. Step 2 is to perform image dilation (`imdilate`) on the result of step 1 using the same structural element, and the last step is to subtract the output of step 2 from the original raw image.

# S12 Light field refocusing

Light field refocusing is a backprojection algorithm for light field measurements. We implement this using a "shift-and-add" algorithm by the following equation:

$$RFV(x, y, \Delta z) = \sum_{u=-1}^{+1} \sum_{v=-1}^{+1} VS(u, v; x - \frac{M^2 d}{z_0} u\Delta z, y - \frac{M^2 d}{z_0} v\Delta z) \tag{13}$$

where $RFV(x, y, \Delta z)$ is the refocused slice with $\Delta z$ refocused distance, $z_0$ is the nominal focal distance from the MLA, $d$ is the diameter of a lenslet in the MLA, $M$ is the magnification of the imaging system, $VS$ is the stack of cropped tomographic views, and $(u, v)$ is the coordinates of the 3x3 MLA (i.e. $VS(-1, -1; \cdot, \cdot)$ is the 512x512 cropped top left view, $VS(0, 0; \cdot, \cdot)$ is the cropped center view, etc).

## S13 Detection metrics

The F1 score is our measure of performance for our reconstruction algorithms, which we perform on synthetic test data. F1 score is defined as

$$\text{F1 score} = 2\frac{\text{precision} \cdot \text{recall}}{\text{precision} + \text{recall}} \tag{14}$$

where precision is defined as # true positives / (# true positives + # false positives) and recall is defined as # true positives / (# true positives + # false negatives).

We compute precision and recall slice-wise as well as for the entire volume by solving the linear assignment problem using MATLAB's built-in `matchpairs` function. The 3D locations of the emitters are known for the ground truth, and the locations for the emitters in the reconstruction are computed by using the MATLAB function `bwconncomps` on thresholded binary reconstruction and then the emitter locations are given using the MATLAB function `regionprops`. Emitters that have fewer than 3 pixels are discarded to account for noise in the reconstruction. We carry out F1 score calculations using five threshold values, (0.1, 0.3, 0.5, 0.7, 0.9) and we use the result with the highest F1 score.

## S14 Confocal microscopy

The Olympus FV3000 laser scanning confocal microscope was used to measure all scattering phantoms and the fixed brain slice. We used a 10x objective with numerical aperture of 0.4. The laser had a wavelength of 488 nm operating at a power of 1.94 mW for all depths. The detector high voltage (HV) was set to 350 V, an offset of 4 V, and digital gain 1x. The final measurement was performed by collecting 2x2 tiles with a 100$\mu$m overlap. Each tile was acquired using a 50$\mu$m pinhole with a dwell time of 2 µs, a pixel sampling of 512x512 over a 1279$\mu$m x 1279$\mu$m FOV and an axial step size of 3$\mu$m. All three phantoms and the fixed brain slice were measured with the same parameters except the number of axial slices, which were 51, 96, and 146, in order of increasing scattering length, and 30 for the brain slice.

# References


[1] O. Mengual, G. Meunier, I. Cayré, K. Puech, and P. Snabre, "TURBISCAN MA 2000: multiple light scattering measurement for concentrated emulsion and suspension instability analysis," *Talanta*, vol. 50, no. 2, pp. 445–456, 1999.

[2] "", "Mie scattering calculator."

[3] S. I. Al-Juboori, A. Dondzillo, E. A. Stubblefield, G. Felsen, T. C. Lei, and A. Klug, "Light scattering properties vary across different regions of the adult mouse brain," *PLOS ONE*, vol. 8, no. 7, p. e67626, 2013. Publisher: Public Library of Science.

[4] Y. Xue, I. G. Davison, D. A. Boas, and L. Tian, "Single-shot 3d wide-field fluorescence imaging with a computational miniature mesoscope," *Science Advances*, vol. 6, no. 43, p. eabb7508, 2020. Publisher: American Association for the Advancement of Science.

[5] Y. Xue, Q. Yang, G. Hu, K. Guo, and L. Tian, "Deep-learning-augmented computational miniature mesoscope," *Optica*, vol. 9, no. 9, pp. 1009–1021, 2022. Publisher: Optica Publishing Group.

[6] K. He, X. Zhang, S. Ren, and J. Sun, "Delving deep into rectifiers: Surpassing human-level performance on ImageNet classification."

[7] S. Boyd, "Distributed optimization and statistical learning via the alternating direction method of multipliers," *Foundations and Trends® in Machine Learning*, vol. 3, no. 1, pp. 1–122, 2010.

[8] N. Antipa, G. Kuo, R. Heckel, B. Mildenhall, E. Bostan, R. Ng, and L. Waller, "DiffuserCam: lensless single-exposure 3d imaging," *Optica*, vol. 5, no. 1, pp. 1–9, 2018. Publisher: Optica Publishing Group.

[9] "https://github.com/bu-cisl/computational-miniature-mesoscope-CM2."
